# Supplementary material for: Characterization of Hydrogen Plasma Defined Graphene Edges
Source: arXiv:1903.07002 ancillary file (2019-03-16)
Supplement: Supplementary file 1 [file supplementary.pdf]

Supplementary Information

# Characterization of Hydrogen Plasma Defined Graphene Edges

Mirko K. Rehmann,[1,*] Yemliha B. Kalyoncu,[1,*] Marcin Kisiel,[1]
Nikola Pascher,[2] Franz J. Giessibl,[3] Fabian Müller,[1] Kenji Watanabe,[4]
Takashi Taniguchi,[4] Ernst Meyer,[1] Ming-Hao Liu,[5,†] and Dominik M. Zumbühl[1,‡]

[1]*Department of Physics, University of Basel, CH-4056 Basel, Switzerland*

[2]*Nanosurf AG, Gräubernstrasse 12, 4410 Liestal, Switzerland*

[3]*Department of Physics, University of Regensburg, 93053 Regensburg, Germany*

[4]*National Institute for Material Science, 1-1 Namiki, Tsukuba 305-0044, Japan*

[5]*Department of Physics, National Cheng Kung University, Tainan 70101, Taiwan*

[*] M. K. R. and Y. B. K. contributed equally to this work

[†] minghao.liu@phys.ncku.edu.tw

[‡] dominik.zumbuhl@unibas.ch

# S1 High quality bulk graphene after hydrogen plasma exposure

In order to investigate the influence of remote hydrogen (H) plasma exposure on the graphene flake, we recorded Raman maps (see Fig. S1). In panel a) and b) we show the integrated 2D- and D-peak intensities, respectively. It is nicely visible, that the D-peak intensity is only high at the edges of the flake and the hexagons and very low in the bulk, showing that exposure of graphene to remote H plasma only edges from defects and the edges and leaves the bulk intact. Furthermore, we can exclude hydrogenation of bulk graphene because this would lead to D-peak intensity[1]. Panel c) shows an AFM height image of the region where the Raman maps in a) and b) were recorded. The green, red and purple crosses are drawn at the same location on the flake through a) - c), namely the green cross lays inside the hexagon, the red cross at the edge and the purple cross on bulk graphene.

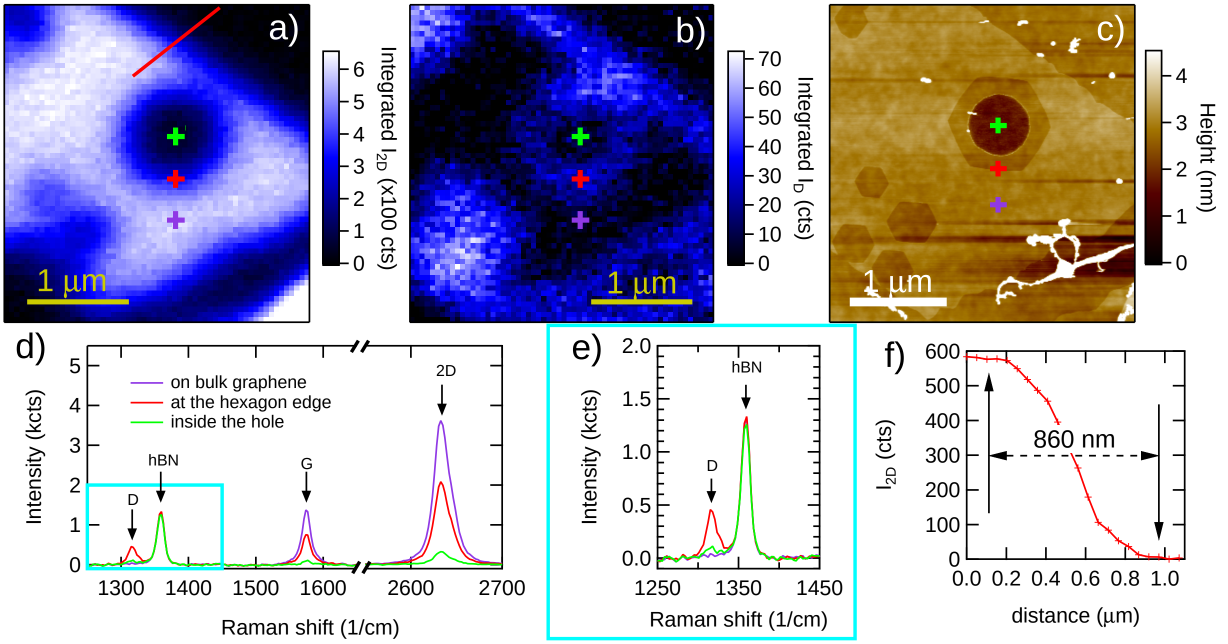


FIG. S1. **High quality bulk graphene after H plasma exposure** Integrated 2D-intensity (a)) and integrated D-peak intensity (b)) of a section of a single layer (SL) graphene flake on a hexagonal boron nitride (hBN) substrate after 4 h of H plasma exposure. c) AFM height image of the region where the Raman maps in a) and b) were recorded. d) Raman spectra recorded at the locations indicated by the colored crosses in a) - c). e) Zoom-in on the region of the D-peak. f) 2D-peak intensity as a function of distance measured along the red solid line in panel a).

Raman spectra were recorded at the location of these crosses and are shown in panel d) with the corresponding color coding. We observe the graphene related D-, G-, and 2D-peaks, as well as the hBN-peak coming from the substrate. Looking at the G- and 2D-peaks, the intensity is highest for the measurement on bulk graphene, decreases to about half the intensity for the measurement at the hexagon edge and almost vanishes for the measurement taken inside the hexagon. Since the laser spot size is on the order of the hexagon size, the G- and 2D-peak intensities do not fully vanish because the tails of the Gaussian beam shape still excite a small fraction of graphene. Interestingly, the D-peak intensity is only high for the measurement taken at the edge and zero inside and outside the hexagon (see panel e) for the zoom-in). This shows, that the rim initially created when the starting defect was fabricated by reactive ion etching (RIE) in an $Ar/O_2$ plasma does not contribute to the graphene D-band in the Raman spectrum. In Figure S1 f) we show the intensity profile of the 2D-peak, recorded along the red solid line in panel a). From this profile we extract a laser spot diameter of $\sim 860\,\mathrm{nm}$. This is well in agreement with the theoretically expected diffraction-limited spot diameter ($1.22 * \lambda/NA = 858\,\mathrm{nm}$, with the numerical aperture $NA = 0.9$ and the laser wavelength $\lambda = 633\,\mathrm{nm}$).

## S2 Laser power test

A crucial condition for the investigation of the edge constitution by means of Raman spectroscopy is that the edge is not changed upon laser irradiation. Indeed it has been observed experimentally[2] that edge reconstruction due to laser annealing can happen at graphene edges. To ensure, that our graphene edges are not altered upon laser irradiation we performed a laser power test. In Figure S2 a) we show an AFM height image of the sample on which we performed the laser power test. In panel b) we plot the normalized D-peak intensities measured at different stages of the laser power test (measurement # 1 to 5).

First we measured at both hexagons with a laser power of 0.5 mW (measurement # 1). In a second step we expose hexagon 2 five times, each time for 1 min, to a laser power of 1.5 mW (measurement # 2). After this exposure to 1.5 mW we measure again at both hexagons with 0.5 mW (measurement # 3 to 5). Comparing the normalized D-peak intensities recorded before exposure to 1.5 mW (measurement # 1) with the intensities recorded afterwards (measurement # 3 to 5), it is indicated that measuring with a laser power of 1.5 mW does

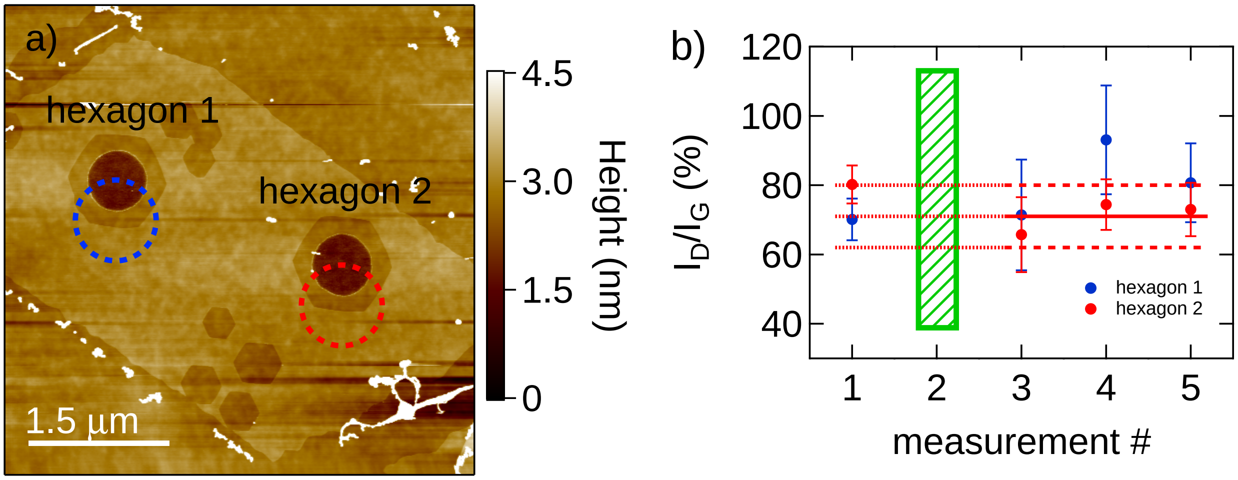


FIG. S2. **Laser power test** a) AFM height image of a SL graphene flake on hBN after 4 h of remote H plasma exposure. The blue and red dashed circles indicate the laser spot where the Raman spectra shown in panel b) were recorded. b) Normalized D-peak intensity recorded at different stages of the laser power test. Measurement # 1, 3, 4 and 5 were acquired with a laser power of 0.5 mW. Only hexagon 2 was exposed to a laser power of 1.5 mW, see measurment # 2 (green dashed area indicates exposure to 1.5 mW). The red solid and dashed lines at measurement # 3 to 5 indicate the average and the standard deviations, respectively. They are prolonged to the left across measurement # 1 and 2 and show that the normalized D-peak intensities recorded before and after exposure to 1.5 mW are comparable. All data points are averages over five measurements and the error bars are the corresponding standard deviations.

not change the recorded D-peak intensity significantly and hence the edge is not impaired. Hence we generally measured with a laser power of 1.5 mW to have a reasonable signal to noise ratio.

## S3 Extraction of the cavity length

In order to characterize the electronic quality of our H plasma exposed graphene samples, we extract a lower bound for the mean free path $l_{mfp}$ of the charge carriers from the oscillation period of the Fabry-Pérot oscillations which are only visible if $l_{mfp}$ exceeds the cavity length L. In particular, L can be calculated from the charge carrier density values n of two consecutive oscillations:

$$L = \frac{\sqrt{\pi}}{\sqrt{n_{j+1}} - \sqrt{n_j}} \tag{1}$$

In Figure S3 we present electronic transport data recorded on the sample presented in Figure 5 in the main manuscript. Panel a) shows the conductance as a function of the inner ($n_{in}$) and outer ($n_{out}$) densities, where $n_{in}$ is the density in the top gated area and $n_{out}$ is the density in the graphene which is only influenced by the global back gate. The conductance map can be divided into four regimes: pnp, pp'p, npn and nn'n. In the two bipolar regimes (pnp and npn) pn-junctions are formed which build a cavity for the charge carriers and lead to Fabry-Pérot resonances (see panel b) for a cut along the blue line in a)). Using equation1 we extract values for L at different $n_{out}$, see panel c). The largest cavity sizes are reached for low values of $n_{out}$ and large values of $n_{in}$. In particular, the values for L lay in the range of 160 nm to 330 nm.

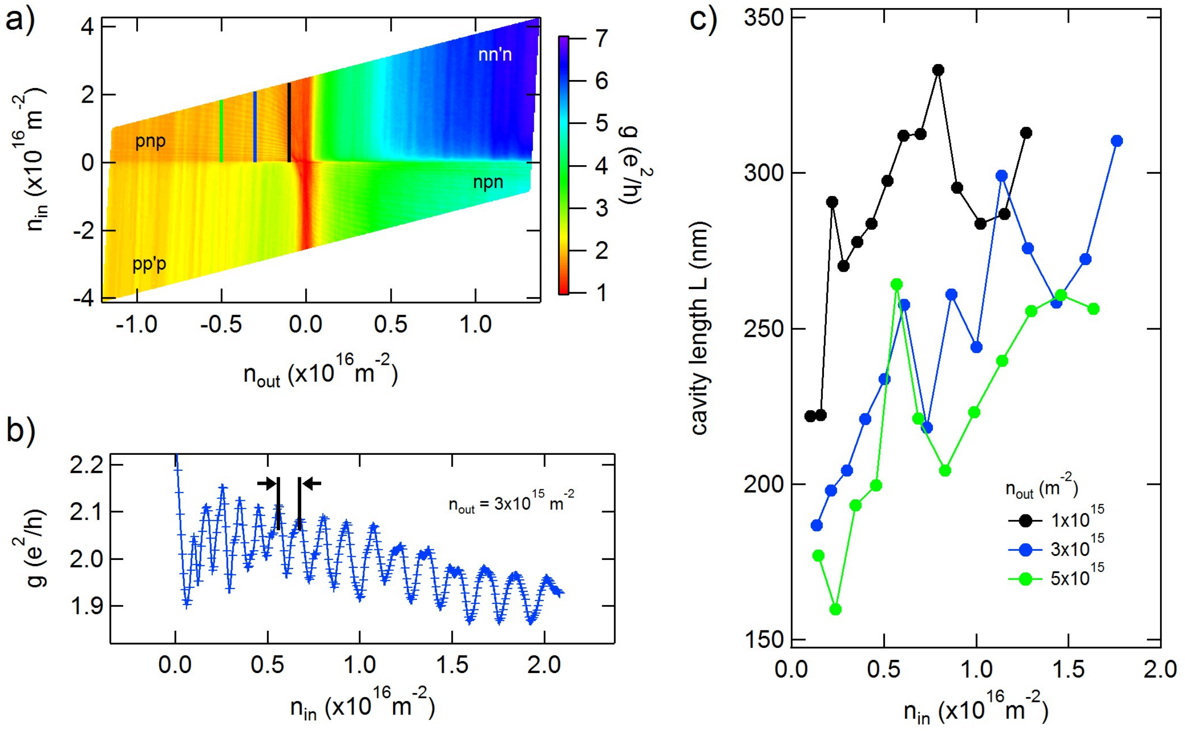


FIG. S3. **Extraction of the cavity length** a) conductance as a function of $n_{in}$ and $n_{out}$. b) cut along the blue solid line in a). Fabry-Pérot resonances are visible indicating ballistic transport between the pn-interfaces. c) Extracted cavity lengths L as a function of $n_{in}$ for three different values of $n_{out}$.

## S4 Edge Reconstruction

Reconstruction of zigzag (ZZ) edges has been observed experimentally[3, 4] and predicted theoretically[5]. Among them, Xu et al.[3] proposed a reconstruction mechanism which leads to four types of edge reconstructions and has the following form:

$$I_D \propto \frac{1}{4}f1 + f2 + \frac{1}{2}f1cos^2(\theta - \phi) \tag{2}$$

where $f_1$ describes the relative weight of armchair (AC)-30° segments, $f_2$ are the point defects, $f_3$ are the ZZ-0° segments and $f_4$ are the ZZ-60° weights. $\theta$ denotes the polarization angle with respect to the edge and $\phi$ is an offset which could stem from an alignment error. Since only AC-30° segments and point defects are D-peak active, it is possible to learn about their relative abundance ($f_1/f_2$) by performing polarized Raman experiments. In Figure S4 a) we plot the normalized D-peak intensity as a function of $\theta$ which was measured at the edge of the hexagon shown in Figure 4 a) in the main manuscript. The blue curve is a fit to equation 2 from which we extract values for $f_1$ and $f_2$. The extracted values indicate that AC-30° segments are much more abundant than point defects and hence that the edge essentially consists only of AC-30° and ZZ segments.

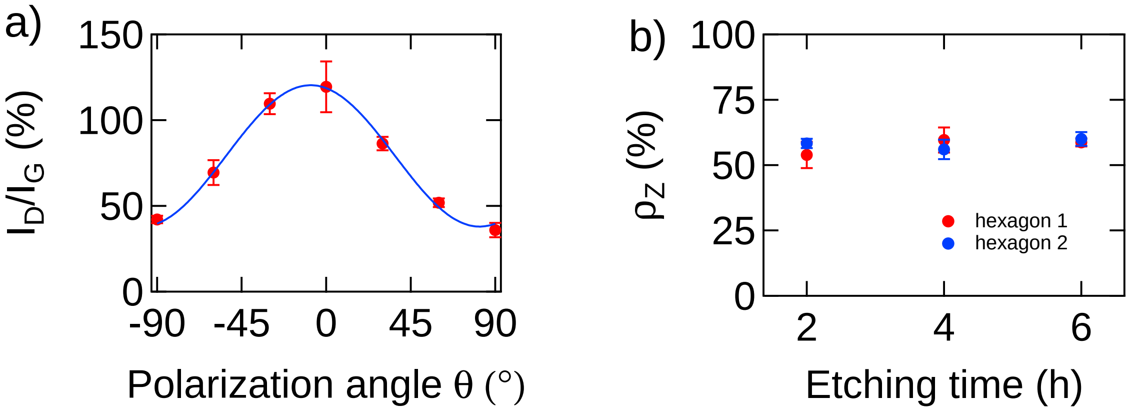


FIG. S4. **Edge reconstruction.** a) Normalized D-peak intensity as a function of the polarization angle $\theta$ for the hexagon shown in Fig. 4 a) of the main manuscript. The blue curve is a fit to equation 2 yielding $f_1 = 165 \pm 6$, $f_2 = -3 \pm 3$ and $\phi = -8 \pm 1$. b) $\rho_Z$ as a function of etching time for two different hexagon edges.

In Figure S4 b) we plot the ratio of ZZ to AC-30° segments $\rho_Z$ extracted at different stages of the etching process for two different hexagon edges. The extraction of $\rho_Z$ was done following the procedure presented in ref. 6 as also described in the main manuscript. Within the experimental error bars $\rho_Z$ is similar for all investigated etching times.

## S5 Effect of the Hole Shape on the D-peak Intensity

As complementary to the discussion of the etching series presented in Figure 3 of the main manuscript, the geometrical change from the circular hole to the hexagonal hole must be taken into account in order to interpret the increase of the D-peak intensity correctly. Typically, a change in edge length effects the D-peak intensity and a change in the graphene area enclosed in the laser spot effects the G-peak intensity. These shape changes must be normalized such that $I_D/I_G$ only manifests the edge quality.

First, we look at the change of the shape from the RIE circular hole to the H plasma etched hexagonal hole. The total edge length enclosed in the laser spot for both shapes are almost equal to each other ($\sim 940\,\mathrm{nm}$). But for the total D-peak intensity, it is crucial to consider the polarization direction of the light with respect to the orientation of the edge and the Gaussian intensity profile of the laser spot. We calculate an effective D-peak intensity by assuming that every point at the edge allows the second order scattering process which is responsible for the D-peak signal. This assumption assures that the following calculation only represents the geometrical changes from a circular shape to a hexagonal shape. When the laser spot is positioned as seen in Figure S5,the D-peak intensity in a single spectrum measurement is given by:

$$I_D \approx \int \int d\beta dr P(\beta) \cos^2(\theta + \beta) I(\vec{r}). \tag{3}$$

The polarization function, $P(\beta)$, determines the laser power at an angle $\beta$ with respect to the horizontal axis, shown in Figure S5. For linear polarization, this function is maximum at the polarization angle and zero at 90 degrees from the polarization angle. For general elliptical polarizations, the function is written explicitly in equation 4, describing laser power for each angle in our single spectrum measurements:

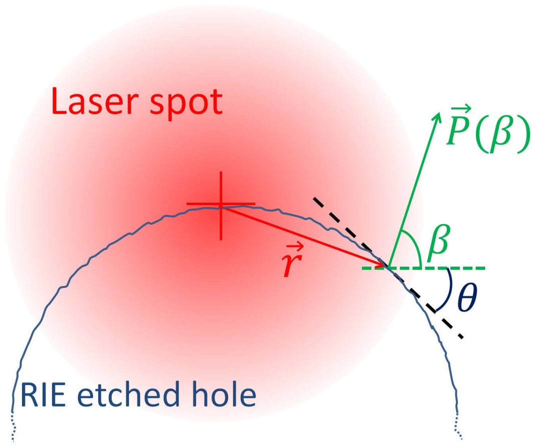


FIG. S5. **Schematic for the integral in equation 3** In a single spectrum measurement, the center of the laser spot is located at the circumference. For any point along the edge, the distance from the center of the laser spot is defined as $\vec{r}$. The polarization vector $\vec{P}(\beta)$, is defined with angle $\beta$ with respect to the horizontal axis (green dashed line). The orientation of the edge, which is the tangent line at that point, is also defined with respect to the horizontal axis with angle $\theta$.

$$|\vec{P}(\beta)| = P(\beta) = \sqrt{(2.5\cos\beta)^2 + \sin^2(\beta)}. \tag{4}$$

The coefficient (2.5) describes how much the polarization is deviated from a perfect circular polarization due to an asymmetry at the beam splitter. For the circular polarization, $\beta$ is integrated from 0 to $\pi$. The second function $I(\vec{r})$ describes the Gaussian beam shape:

$$I(\vec{r}) = I_0 e^{-2\frac{r^2}{\omega_0^2}} \tag{5}$$

with $\vec{r}$ being the radial distance from the center of the laser spot to the respective point at the edge and $\omega_0$ being the (Gaussian) beam waist, measured and calculated to be 430 nm. The third part is the cosine squared function which is a correction due to that the D-peak intensity is maximum (minimum) when the polarization direction is parallel (perpendicular) to the edge direction. The argument of this function is the sum of the polarization angle $\beta$ and the angle $\theta$ of the tangent line with respect to the horizontal axis, as shown in Figure S5.

In order to calculate the effective D-peak intensity at the RIE hole, we apply this integral onto the circumference of the circular hole that fits inside the laser spot, as drawn in Figure S5. For ease-of-calculation, the full circular shape is approximated as a 60-edge-polygon which has an imperceptible effect on the calculation. It should also be noted that for the

calculation with the right integral limits, the integral in equation 3 is converted into a line integral which runs along the circumference enclosed by the laser spot.

Secondly, we calculate the effective D-peak intensity for the hexagonal hole. This calculation is easier than the circular case since it includes only 3 edge segments with angles of 0 and ±60 degrees. The lengths of the hexagonal hole edges are measured on AFM images and all the dimensions of the holes and the D-peak intensity calculations are given in Table I.

Then we calculate the graphene area enclosed in the laser spot. Obviously, the graphene area enclosed in the laser spot changes from circular to hexagonal hole. Since we locate the center of the laser spot at the center of the top or bottom edge, half of the laser spot always covers the same graphene area but only the side pieces around the hole are different after each etching step. At this point, we calculate the area by using simple geometry and write the result again in Table I. As you can see the change in area is at most 14 %. In this calculation, we assume that the G-peak intensity is only proportional to the area of graphene enclosed in the laser spot and we do not consider the Gaussian intensity profile. In fact, the effect of these side areas on the G-peak intensity is much less than the calculated values since they are further away from the center.

The resulting $I_D/I_G$ ratios are given in Table I. All the values in the table are normalized to the value for the RIE hole of the corresponding quantity. As a result, the top row (RIE hole values) is always equal to 1 and the values for 2h etching and 4h etching show the relative change from the RIE case. Apparently, the calculated $I_D/I_G$ due to the geometrical change of the edge length and the area (rightmost column) does not correspond to the measured values of $I_D/I_G$ in the main text. This means that the increase of the $I_D/I_G$ values from the RIE hole to the H plasma etched hole is not due to that the edge is longer or the graphene area is less but it is due to a change in the atomic configuration at the edge. In other words, compared to an RIE etched edge of the same length, an H plasma etched edge has more AC edge segments contributing to the D-peak signal.

| Etching (x) | Total edge length inside $\omega_0$ | Calculated $I_D^x/I_D^{RIE}$ | Area inside $\omega_0$ $\approx I_G^x/I_G^{RIE}$ | Measured $I_D^x/I_G^x$ (main text) | Calculated $I_D^x/I_G^x$ (geometry) |
|---|---|---|---|---|---|
| RIE | $\sim 940nm$ | 1 | 1 | 1 | 1 |
| 2h H-plasma | $\sim 945nm$ | 1.03 | 0.89 | 2.4 | 1.16 |
| 4h H-plasma | $\sim 950nm$ | 1.04 | 0.86 | 2.4 | 1.21 |

TABLE I. Calculations for the 600 nm hole with circularly polarized light

## S6 Electronic Mobility of Encapsulated Hall Bar

In this section we present transport data recorded on a SL graphene Hall bar encapsulated between two hBN flakes. In particular we are interested in the cleanliness of the encapsulated graphene and extract the mean free path $l_{mfp}$ of the charge carriers to compare it with relevant length scales of the investigated graphene nano ribbon (GNR) devices discussed in the main manuscript (Fig. 7). In Figure S6 a) an optical microscopy image of the encapsulated Hall bar is shown with the electronic circuit drawn on top of it. In panel b) the conductivity $\sigma$ as a function of the charge carrier density $n$ is plotted. The blue and green curves are fits to the following equation:

$$\sigma(n) = \left(\frac{1}{\mu n e} + \rho_s\right)^{-1} \tag{6}$$

where $\mu$ is the mobility, e the electronic charge and $\rho_s$ a series resistivity which is composed of the contact resistances and the cryostat lead resistances. The fit to the electron side (green curve) gives $\mu = 134'000\,\mathrm{cm}^2/\mathrm{Vs}$ and the fit to the hole side (blue curve) gives $\mu = 114'000\,\mathrm{cm}^2/\mathrm{Vs}$. In panel c) we plot $\sigma$ as a function of $n$ on a log-log scale. By looking at the position of the kink, indicated by the black solid and dashed lines, we extract an estimate of the residual disorder density which is $3 \cdot 10^{10}\,\mathrm{cm}^{-2}$. Further, we calculate $l_{mfp}$ of the charge carriers for the electron side by using the following formula:

$$l_{mfp}(\mu, n) = \frac{\hbar}{e} \cdot \mu \cdot \sqrt{\pi n} \tag{7}$$

where $\hbar$ is the Planck constant.

The mean free path reaches $1\,\mu$m at $n = 4.1 \cdot 10^{11}\,\mathrm{cm}^{-2}$ which clearly exceeds all relevant length scales in the GNR devices discussed in the main manuscript (Fig. 7).

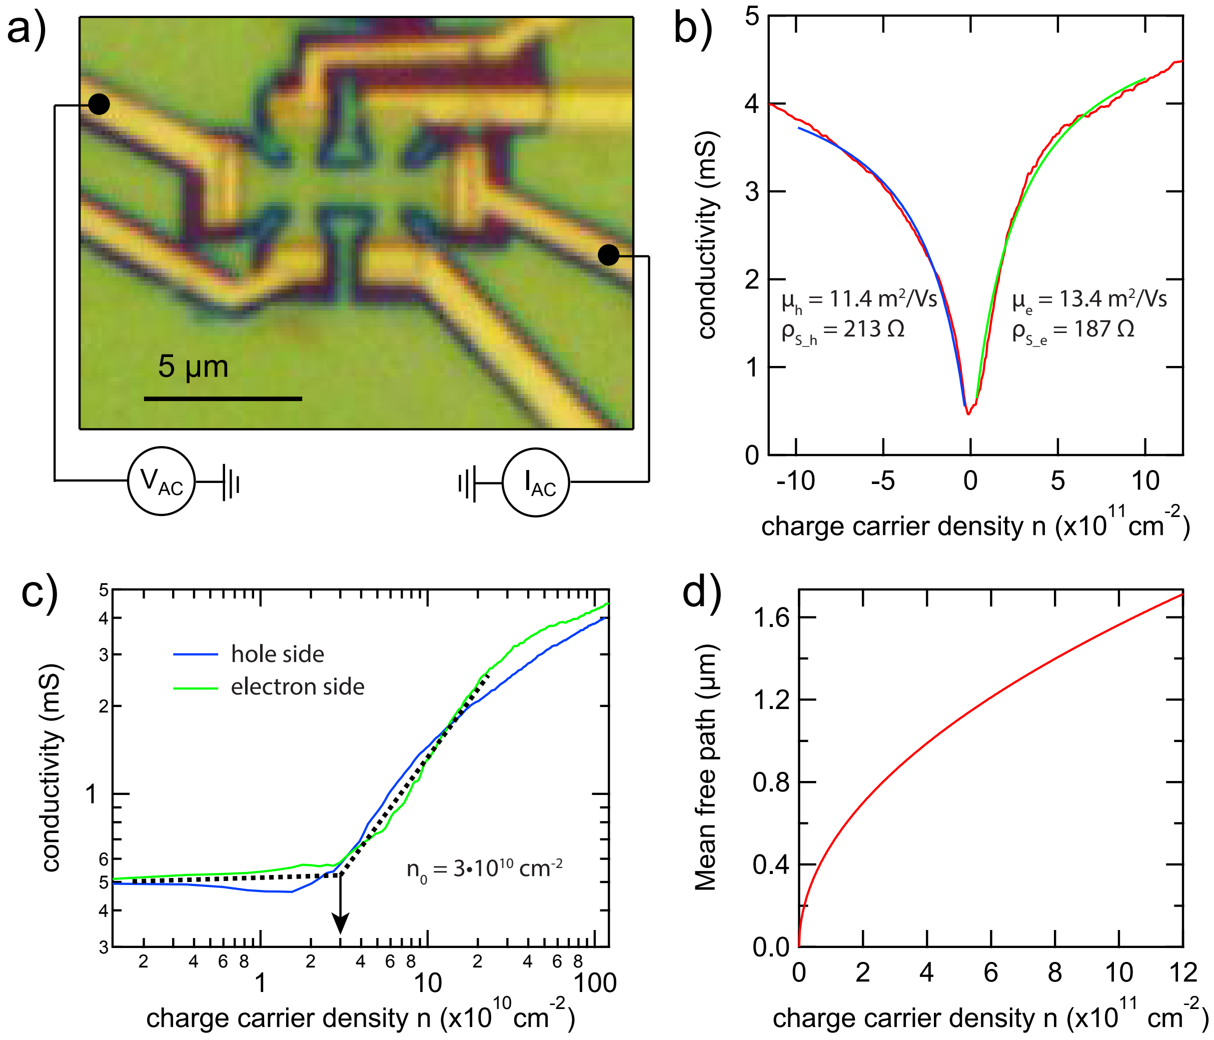


FIG. S6. **Mobility of an Encapsulated Hall Bar** a) Optical microscopy image of the investigated SL graphene Hall bar encapsulated between two hBN flakes. The side contacts are yellow and the electronic circuit is indicated. b) Conductivity as a function of the charge carrier density. The green and blue curves are fits to equation 6. The following fitting parameters were obtained: electron side, $\mu_e = 1.34 \cdot 10^5 \pm 1 \cdot 10^3\,\mathrm{cm}^2/\mathrm{Vs}$, $\rho_{S\_e} = 187 \pm 1\,\Omega$; hole side: $\mu_h = 1.14 \cdot 10^5 \pm 1 \cdot 10^3\,\mathrm{cm}^2/\mathrm{Vs}$, $\rho_{S\_h} = 213 \pm 1\,\Omega$. c) Conductivity as a function of the absolute value of the charge carrier density plotted in a log-log representation. The location of the kink gives the estimate of the residual disorder density $\mathrm{n}_0$ which is $3 \cdot 10^{10}\,\mathrm{cm}^{-2}$. d) Mean free path as a function of the charge carrier density for the mobility value obtained for the electron side.

## S7 Comparison of the Experiment with the Simulation

In this section, the differences between the experimentally measured conductance $g(\Delta x_{\text{np-exp}})$ and the simulated conductance $g(\Delta x_{\text{np-sim}})$ are discussed. In the experiment, the positions of the two pn-interfaces can be tuned with gate voltages applied to the local top gate and the global back gate. Thereby, the pn-interfaces move always in opposite directions, i.e. either towards each other or apart from each other, see Figure S7 a). In the simulation, on the other hand, the two pn-interfaces move always in the same direction, see Figure S7 b).

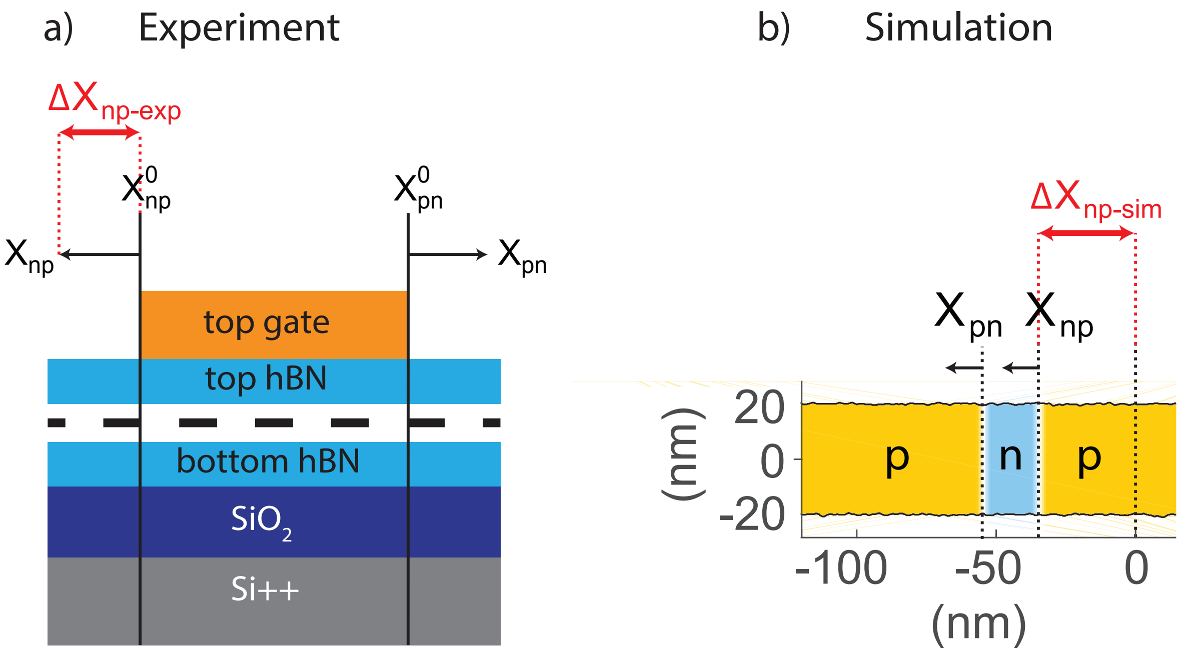


FIG. S7. **Experiment vs Simulation** a) Schematic of the cross section of the device on which transport was measured. b) Model which was used for the simulations.

This is equivalent to connecting an *np* junction with conductance $G(x_{\text{np}})$ and a *pn* junction with conductance $G(x_{\text{pn}})$ in series, and then move the two junctions together in the same direction. Specifically, we are comparing our simulations for

$$g(\Delta x_{\text{np-sim}}) = g(x_{\text{np}}) \propto G(x_{\text{pn}})G(x_{\text{np}})$$

with the experimentally measured

$$g(\Delta x_{\text{np-exp}}) = g(x_{\text{np}} - x^0_{\text{np}}) \propto G(x_{\text{np}} - x^0_{\text{np}})G(x_{\text{pn}} - x^0_{\text{pn}}) \; ,$$

where $x^0_{\text{np}} = -100\,\text{nm}$ and $x^0_{\text{pn}} = 100\,\text{nm}$ are the designed positions of the two edges of the top gate, and $x_{\text{pn}} = -x_{\text{np}}$ due to their opposite movement. Despite this subtle difference, the

comparison makes reasonably good sense because the AC-30° segments of the edge disorder are randomly located. That is, in the simulation, $G(x_{\text{pn}})$ is expected to be uncorrelated with $G(x_{\text{np}})$, just like in the experiment, $G(x_{\text{np}} - x^0_{\text{np}})$ is expected to be uncorrelated with $G(x_{\text{pn}} - x^0_{\text{pn}})$, either. Hence, $g(\Delta x_{\text{np-exp}}) \sim g(\Delta x_{\text{np-sim}})$ and therefore we introduce the parameter $\Delta x_{\text{np}}$ for both, experiment and simulation, as used in the main paper in Figure 5 and Figure 6.

## S8 Conversion of Backgate Voltage to the pn-interface Location

In order to interpret the valley-isospin oscillations in terms of the pn-interface locations it is necessary to convert gate voltages to the actual pn-interface locations. In Figure S8 a) a calculation of the electrostatics of the studied device is shown where the pn-interface position relative to the left edge of the top gate $\Delta X_{np}$ is plotted as a function of back gate and top gate voltages. In panel b) a cut along the red solid line in a) is shown. This curve was used to convert back gate voltage to $\Delta X_{np}$ for the curves presented in the main manuscript.

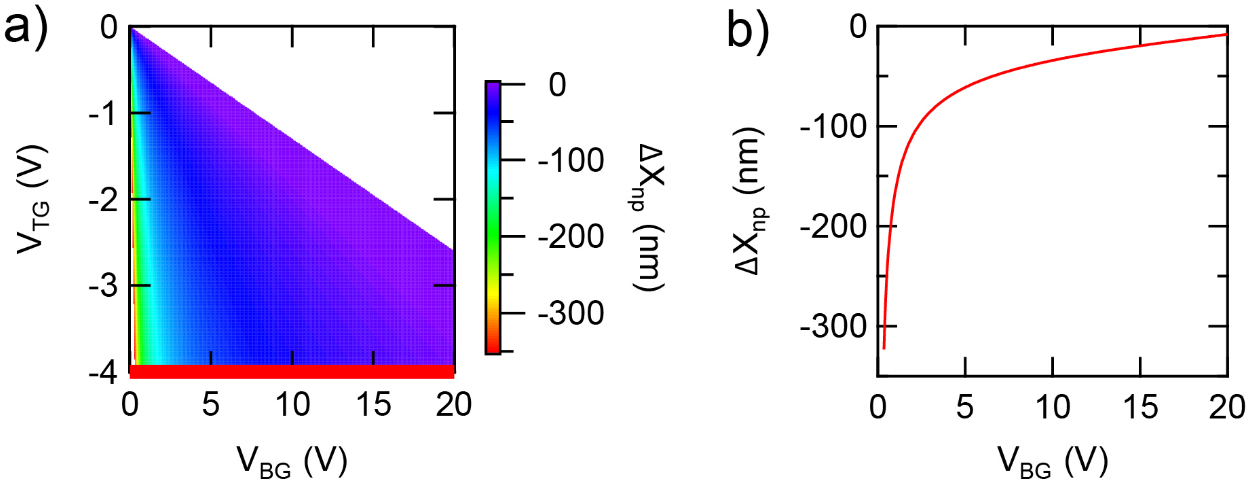


FIG. S8. **Conversion of Backgate Voltage to the pn-interface Location** a) Electrostatic simulation of the device presented in Figure 5 in the main manuscript where the pn-interface location relative to the left edge of the top gate $\Delta X_{np}$ is plotted as function of top and back gate voltages. b) Cut along the red solid line in a).

## A. REFERENCES

---


[1] D. C. Elias, R. R. Nair, T. Mohiuddin, S. Morozov, P. Blake, M. Halsall, A. Ferrari, D. Boukhvalov, M. Katsnelson, A. Geim, *et al.* *Control of graphene's properties by reversible hydrogenation: evidence for graphane.* Science **323**, 610 (2009).

[2] M. Begliarbekov, K.-I. Sasaki, O. Sul, E.-H. Yang, and S. Strauf. *Optical control of edge chirality in graphene.* Nano letters **11**, 4874 (2011).

[3] Y. N. Xu, D. Zhan, L. Liu, H. Suo, Z. H. Ni, T. T. Nguyen, C. Zhao, and Z. X. Shen. *Thermal Dynamics of Graphene Edges Investigated by Polarized Raman Spectroscopy.* ACS Nano **5**, 147 (2011). PMID: 21171568.

[4] K. He, A. W. Robertson, Y. Fan, C. S. Allen, Y.-C. Lin, K. Suenaga, A. I. Kirkland, and J. H. Warner. *Temperature Dependence of the Reconstruction of Zigzag Edges in Graphene.* ACS Nano **9**, 4786 (2015). PMID: 25880335.

[5] P. Koskinen, S. Malola, and H. Häkkinen. *Self-Passivating Edge Reconstructions of Graphene.* Phys. Rev. Lett. **101**, 115502 (2008).

[6] C. Casiraghi, A. Hartschuh, H. Qian, S. Piscanec, C. Georgi, A. Fasoli, K. Novoselov, D. Basko, and A. Ferrari. *Raman spectroscopy of graphene edges.* Nano letters **9**, 1433 (2009).
